# Supplementary material for: Local Distribution Obfuscation via Probability Coupling
Source: arXiv:1907.05991 source file (2019-09-30)
Supplement: Supplementary file 1 [file _appendix-full-tables.tex]

\begin{table*}[h]
  \centering
  \caption{Summary of basic properties of distribution privacy.}
  \label{table:summary:basic-properties:DistP:all}
  
  \footnotesize
  \begin{tabular}{lll}
    \hline
    & Distribution privacy \\
    \hline
    Sequential composition $\Seq$ ($\Dinf^{\delta}$) &
      $\alg_b$ is $(\varepsilon_b,\Dinf^{\delta_b})$-\DistP{} \\
    &
      $\Rightarrow$
      $\alg_1 \Seq \alg_0$ is $(\varepsilon_0+\varepsilon_1, \Dinf^{(\delta_0+\delta_1)\cdot|\varPhi|})$-\DistP{} \\
    \hline
    Sequential composition $\liftSeq$ ($\Dinf^{\delta}$) &
      $\alg_b$ is $(\varepsilon_b,\Dinf^{\delta_b})$-\DistP{} \\
    &
      $\Rightarrow$
      $\alg_1 \liftSeq \alg_0$ is $(\varepsilon_0+\varepsilon_1, \Dinf^{\delta_0+\delta_1})$-\DistP{} \\
    \hline
    Sequential composition $\Seq$ ($\DKL$) &
      $\alg_b$ is $(\varepsilon_b,\DKL)$-\DistP{} \\
    &
      $\Rightarrow$
      $\alg_1 \Seq \alg_0$ is $(\varepsilon_0+\varepsilon_1, \DKL)$-\DistP{} \\
    \hline %\hline
    Sequential composition $\liftSeq$ ($\DKL$) &
      $\alg_b$ is $(\varepsilon_b,\DKL)$-\DistP{} \\
    &
      $\Rightarrow$
      $\alg_1 \liftSeq \alg_0$ is $(\varepsilon_0+\varepsilon_1, \DKL)$-\DistP{} \\
    \hline %\hline
    Post-processing ($D = \Dinf^{\delta}$, $\Df$) &
      $\alg_0$ is $(\varepsilon,D)$-\DistP{}
      $\Rightarrow$
      $\alg_1\circ\alg_0$ is $(\varepsilon,D)$-\DistP{} \\
    \hline
    Pre-processing (by $c$-stable $T$) &
      $\alg$ is $(\varepsilon,D)$-\DistP{}
      $\Rightarrow$
      $\alg\circ T$ is $(c\,\varepsilon,D)$-\DistP{} \\
    \hline
  \end{tabular}
\end{table*}

\begin{table*}[h]
  \centering
  \caption{Summary of basic properties of extended distribution privacy.}
  \label{table:summary:basic-properties:XDistP:all}
  \footnotesize
  
  \begin{tabular}{lll}
    \hline
    & Extended distribution privacy \\
    \hline
    Sequential composition $\Seq$ ($\Dinf^{\delta}$) &
      $\alg_b$ is $(\varepsilon_b,\sensinf,\Dinf^{\delta_b})$-\XDistP{} \\
    &
      $\Rightarrow$
      $\alg_1 \Seq \alg_0$ is $(\varepsilon_0+\varepsilon_1, \sensinf, \Dinf^{(\delta_0+\delta_1)\cdot|\varPhi|})$-\XDistP{} \\
    \hline
    Sequential composition $\liftSeq$ ($\Dinf^{\delta}$) &
      $\alg_b$ is $(\varepsilon_b,\sensinf,\Dinf^{\delta_b})$-\XDistP{} \\
    &
      $\Rightarrow$
      $\alg_1 \liftSeq \alg_0$ is $(\varepsilon_0+\varepsilon_1, \sensinf, \Dinf^{\delta_0+\delta_1})$-\XDistP{} \\
    \hline
    Sequential composition $\Seq$ ($\DKL$) &
      $\alg_b$ is $(\varepsilon_b,\sensemd,\DKL)$-\XDistP{} \\
    &
      $\Rightarrow$
      $\alg_1 \Seq \alg_0$ is $(\varepsilon_0+\varepsilon_1, \sensemd, \DKL)$-\XDistP{} \\
    \hline %\hline
    Sequential composition $\liftSeq$ ($\DKL$) &
      $\alg_b$ is $(\varepsilon_b,\sensemd,\DKL)$-\XDistP{} \\
    &
      $\Rightarrow$
      $\alg_1 \liftSeq \alg_0$ is $(\varepsilon_0+\varepsilon_1, \sensemd, \DKL)$-\XDistP{} \\
    \hline %\hline
    Post-processing ($D = \Dinf^{\delta}$, $\Df$) &
      $\alg_0$ is $(\varepsilon,\sensfunc,D)$-\XDistP{}
      \!$\Rightarrow$\!
      $\alg_1{\circ}\alg_0$ is $(\varepsilon,\sensfunc,D)$-\XDistP{} \\
    \hline
    Pre-processing (by $c$-stable $T$) &
      $\alg$ is $(\varepsilon,\sensfunc,D)$-\XDistP{}
      \!$\Rightarrow$\!
      $\alg\circ T$ is $(c\,\varepsilon,\sensfunc,D)$-\XDistP{} \\
    \hline
  \end{tabular}
\end{table*}
